# Supplementary material for: Optimal Rates for Federated Variational Inequalities under different relaxations of bounded variance assumption
Source: arXiv:2610.12641 source file (2026-10-08)
Supplement: Supplementary file 1 [file contents.tex]

\makeatletter
\section*{Appendix contents}
\begingroup
\small
\setcounter{tocdepth}{3}
\renewcommand*\l@section[2]{%
  \ifnum\c@tocdepth>\z@
    \addpenalty\@secpenalty
    \addvspace{.7em\@plus\p@}%
    \setlength\@tempdima{2em}%
    \begingroup
      \parindent\z@ \rightskip\@pnumwidth
      \parfillskip-\@pnumwidth
      \leavevmode\bfseries
      \advance\leftskip\@tempdima \hskip-\leftskip
      #1\nobreak\hfil\nobreak
      \hb@xt@\@pnumwidth{\hss #2}\par
    \endgroup
    \penalty\@M
  \fi}
\renewcommand*\l@subsection{\@dottedtocline{2}{2em}{3em}}
\renewcommand*\l@subsubsection{\@dottedtocline{3}{5em}{3.5em}}
\hypersetup{linktoc=all}
\@starttoc{aptoc}
\endgroup
% Record appendix headings separately while preserving the PDF bookmarks.
\let\appendix@addcontentsline\addcontentsline
\renewcommand{\addcontentsline}[3]{%
  \appendix@addcontentsline{#1}{#2}{#3}%
  \def\appendix@entrytype{#1}%
  \def\appendix@tocname{toc}%
  \ifx\appendix@entrytype\appendix@tocname
    \addtocontents{aptoc}{%
      \protect\contentsline{#2}{#3}{\thepage}{\@currentHref}\protected@file@percent}%
  \fi
}
\makeatother
\clearpage
